# Supplementary material for: Spin Frustration and a `Half Fire, Half Ice' Critical Point from Nonuniform $g$-Factors
Source: arXiv:1510.00030 source file (2016-05-10)
Supplement: Supplementary file 1 [file yin_SI.pdf]

# [Supplemental Materials]
# Spin Frustration and a 'Half Fire, Half Ice' Critical Point from Nonuniform $g$-Factors

Wei-Guo Yin *et al.*[*]
*Condensed Matter Physics and Materials Science Division,*
*Brookhaven National Laboratory, Upton, New York 11973, USA*
(Dated: May 10, 2016)

I. Staggered $g$-Factors ($-g_B > g_A > 0$) in Real Materials
II. The Transfer Matrix Method
  A. Thermodynamical observables
  B. Correlations functions
  C. Sublattice magnetization
  D. The zero-temperature limit
    1. $-g_B > g_A > 0$
    2. $-g_B = g_A$

## I. STAGGERED $g$-FACTORS ($-g_B > g_A > 0$) IN REAL MATERIALS

Both orbital angular momentum ($\mathbf{L}$) and spin angular momentum ($\mathbf{S}$) of electron contribute to the magnetic moment ($\mathbf{M}_J$) in the following form

$$\begin{aligned} \mathbf{M}_J &= \mathbf{M}_L + \mathbf{M}_S, \\ \mathbf{M}_L &= g_L \mu_B \mathbf{L}, \\ \mathbf{M}_S &= g_S \mu_B \mathbf{S}, \end{aligned} \tag{1}$$

where in atomic physics,

$$\begin{aligned} g_L &= 1, \\ g_S &= 2. \end{aligned} \tag{2}$$

However, strong octahedral crystal field will split the $d$ orbitals into the well separated $e_g$ and $t_{2g}$ energy levels. The $t_{2g}^5$ subsystem such as $Ir^{4+}$ in the copper-iridium oxide $Sr_3CuIrO_6$ can be transformed[1] to an effective $L = 1$ system—upon projecting out the unoccupied $e_g$ levels—in which $|xy, \sigma\rangle$ and $i|yz, \sigma\rangle \pm |zx, \sigma\rangle$ (where $\sigma =\uparrow$ or $\downarrow$ is the spin index) are the new $L_z = 0$ and $\pm 1$ states, respectively, and

$$\begin{aligned} g_L &= -1, \\ g_S &= 2. \end{aligned} \tag{3}$$

Then, strong spin-orbit coupling on the Ir atom generate an effective total angular momentum $J = \frac{1}{2}$ state.

The $g$-factor tensor that relates the total magnetic moment $\mathbf{M}_J$ and the total angular momentum $\mathbf{J} = \mathbf{L} + \mathbf{S}$ is given by

$$\langle J, J_z | \mathbf{M}_J | J, J_{z'} \rangle = g_J^{z,z'} \mu_B \langle J, J_z | \mathbf{J} | J, J_{z'} \rangle, \tag{4}$$

where the effective $J = \frac{1}{2}$ wave vectors $|J, J_z\rangle$ for Ir atoms in $Sr_3CuIrO_6$ are given by[2]

$$|J, \pm\frac{1}{2}\rangle = \frac{1}{\sqrt{p^2+2}} \left[ p|xy, \uparrow\rangle + i|yz, \downarrow\rangle \pm |zx, \downarrow\rangle \right], \tag{5}$$

where $p \approx 0.65$. Hence the longitudinal $g$-factor that couples to the magnetic field along the $z$ direction is

$$\begin{aligned} g_{\mathrm{Ir}}^z = g_J^{z,z} &= \frac{\langle J, \frac{1}{2} | M_z | J, \frac{1}{2} \rangle}{\mu_B \langle J, \frac{1}{2} | J_z | J, \frac{1}{2} \rangle} \\ &= 2 \langle J, \frac{1}{2} | g_L L_z + g_S S_z | J, \frac{1}{2} \rangle \\ &= 2 \frac{2 g_L + \frac{1}{2} g_S (p^2 - 2)}{p^2 + 2} \\ &= 2 \frac{p^2 - 4}{p^2 + 2} \\ &\approx -2.96 \end{aligned} \tag{6}$$

On the other hand, for the $Cu^{2+}$ $3d^9$ or $t_{2g}^6 e_g^3$ configuration, both $\mathbf{L}$ and spin-orbital coupling vanish. Thus,

$$g_{\mathrm{Cu}} = g_S = 2 < -g_{\mathrm{Ir}}^z$$

## II. THE TRANSFER MATRIX METHOD

We extended the transfer matrix method[3] to solve exactly the following one-dimensional Ising model with alternating $g$-factors:

$$H = -J\sum_{i=1}^{N}\sigma_i\sigma_{i+1} - h\sum_{i}^{N} g_i\sigma_i, \tag{7}$$

which corresponds to $N$ spins ($\sigma_i = \pm 1$) in a line with the periodic boundary condition $\sigma_{N+1} = \sigma_1$. $h$ is a uniform longitudinal magnetic field. The chain has two sublattices $A$ and $B$ with $g_i = g_A$ for odd $i$ and $g_i = g_B$ for even $i$. Here, and from now on, $g_A$ means $\mu_B S g_A$ and $g_B$ means $\mu_B S g_B$ for shorthand notation. The terminology of *uniform*, *uniformly staggered*, *nonuniform* $g$-factors stands for $g_A = g_B$, $g_A = -g_B$, and $|g_A| \neq |g_B|$, respectively. The first two cases with $|g_A| = |g_B|$ are essentially the *same* upon the transformation for sites in the $B$-sublattice only, $\sigma_i \to -\sigma_i$, together with the following substitutions: $J \to -J, \quad g_B \to -g_B$.

The partition function is

$$Z(N,h,T) = \sum_{\sigma_1}\cdots\sum_{\sigma_N} e^{-\beta H}, \tag{8}$$

where $\beta = 1/k_B T$; $T$ is temperature and $k_B$ is the Boltzmann constant. In order to carry out the spin sum, we define two matrices $P_{AB}$ and $P_{BA}$ with matrix elements

$$\begin{aligned}\langle\sigma_{i\in A}|P_{AB}|\sigma_{i+1\in B}\rangle &= e^{\beta[J\sigma_i\sigma_{i+1}+\frac{1}{2}h(g_A\sigma_i+g_B\sigma_{i+1})]}\\ \langle\sigma_{i\in B}|P_{BA}|\sigma_{i+1\in A}\rangle &= e^{\beta[J\sigma_i\sigma_{i+1}+\frac{1}{2}h(g_B\sigma_i+g_A\sigma_{i+1})]}\end{aligned} \tag{9}$$

Thus, they are the $2\times 2$ matrices given by

$$P_{AB} = \begin{pmatrix} e^{\beta J+\frac{1}{2}\beta h(g_A+g_B)} & e^{-\beta J+\frac{1}{2}\beta h(g_A-g_B)} \\ e^{-\beta J-\frac{1}{2}\beta h(g_A-g_B)} & e^{\beta J-\frac{1}{2}\beta h(g_A+g_B)} \end{pmatrix} \tag{10}$$

and $P_{BA} = P_{AB}^T$, whose expression can be obtained by swapping the labels $A$ and $B$ in Eq. (10). We then introduce

$$P_{AA} = P_{AB}P_{BA} = \begin{pmatrix} e^{2\beta J+\beta h(g_A+g_B)} + e^{-2\beta J+\beta h(g_A-g_B)} & e^{\beta h g_B} + e^{-\beta h g_B} \\ e^{\beta h g_B} + e^{-\beta h g_B} & e^{2\beta J-\beta h(g_A+g_B)} + e^{-2\beta J-\beta h(g_A-g_B)} \end{pmatrix} \tag{11}$$

and

$$P_{BB} = P_{BA}P_{AB}, \tag{12}$$

whose expression can be obtained by swapping the labels $A$ and $B$ in Eq. (11).

Hence, the partition function becomes

$$\begin{aligned} Z(N,h,T) &= \sum_{\sigma_1}\cdots\sum_{\sigma_N}\langle\sigma_1|P_{AB}|\sigma_2\rangle\langle\sigma_2|P_{BA}|\sigma_3\rangle\cdots\langle\sigma_{N-1}|P_{AB}|\sigma_N\rangle\langle\sigma_N|P_{BA}|\sigma_1\rangle \\ &= \sum_{\sigma_1}\langle\sigma_1|(P_{AB}P_{BA})^{N/2}|\sigma_1\rangle \\ &= \mathrm{Tr}\left((P_{AA})^{N/2}\right) = \mathrm{Tr}\left((P_{BB})^{N/2}\right). \end{aligned} \tag{13}$$

A simple way to carry out the trace is to diagonalize the transfer matrix, $P_{AA}$. The eigenvalues are

$$\begin{aligned}\lambda_\pm = {}& e^{2\beta J}\cosh(\beta h g_A + \beta h g_B) + e^{-2\beta J}\cosh(\beta h g_A - \beta h g_B) \\ &\pm\sqrt{2\cosh^2(\beta h g_A) + 2\cosh^2(\beta h g_B) + e^{4\beta J}\sinh^2(\beta h g_A+\beta h g_B) + e^{-4\beta J}\sinh^2(\beta h g_A - \beta h g_B)}.\end{aligned} \tag{14}$$

Note that for $g_A = -g_B = g$,

$$\lambda_\pm = e^{-2\beta J}\left(\cosh(\beta h g) \pm \sqrt{\sinh^2(\beta h g) + e^{4\beta J}}\right)^2. \tag{15}$$

The eigenvectors of $P_{AA}$ are $|\Psi_{A,+}\rangle$ and $|\Psi_{A,-}\rangle$, respectively. $P_{BB}$ has the same eigenvalues but different eigenvectors $|\Psi_{B,+}\rangle$ and $|\Psi_{B,-}\rangle$. Then,

$$\mathrm{Tr}\left((P_{AA})^{N/2}\right) = \mathrm{Tr}\left((P_{BB})^{N/2}\right) = \lambda_+^{N/2} + \lambda_-^{N/2}. \tag{16}$$

We will be interested in the thermodynamic limit $N \to \infty$. For $\lambda_+ > \lambda_- \geq 0$, $\lambda_+^{N/2} \gg \lambda_-^{N/2}$. Then, the partition function has the single term:

$$Z(N,h,T) \to \lambda_+^{N/2}. \tag{17}$$

Thus, the free energy per site becomes

$$f(h,T) = -\frac{1}{N} k_\mathrm{B} T \ln Z(N,h,T) = -\frac{1}{2\beta} \ln \lambda_+ \tag{18}$$

### A. Thermodynamical Observables

Given the analytic forms of $\lambda_+$ and $f(h,T)$ in Eq. (14) and Eq. (18), one gets to the magnetization per site:

$$m(h,T) = -\frac{\partial f(h,T)}{\partial h} = \frac{1}{2\lambda_+} \frac{\partial \lambda_+}{\partial(\beta h)} \tag{19}$$

which vanishes as $h/T \to 0$, since $\cosh(\beta h) \to 1$ and $\sinh(\beta h) \to 0$. This means that there is no spontaneous magnetization at any finite temperature in the 1D case. Other thermodynamic quantities such as the susceptibility $\chi(h,T)$, entropy $S(h,T)$, specific heat $C_V(h,T)$ are given by the following:

$$\chi(h,T) = \frac{\partial m(h,T)}{\partial h}, \tag{20}$$

$$S(h,T) = -\frac{\partial f(h,T)}{\partial T}, \tag{21}$$

$$C_V(h,T) = T\frac{\partial S(h,T)}{\partial T}. \tag{22}$$

### B. Correlation Functions

The correlation function of interest is

$$\langle \sigma_m \sigma_n \rangle = \frac{1}{Z(N,h,T)} \sum_{\sigma_1} \cdots \sum_{\sigma_m} \cdots \sum_{\sigma_n} \cdots \sum_{\sigma_N} \sigma_m \sigma_n e^{-\beta H}. \tag{23}$$

There are three cases: (i) Both site $m$ and site $n$ belong to the $A$ sublattice, (i) both sites belong to the $B$ sublattice, and (iii) they belong to different sublattices.

Define the $2 \times 2$ matrix

$$\hat{\sigma}_z = \begin{pmatrix} 1 & 0 \\ 0 & -1 \end{pmatrix} \tag{24}$$

(i) Then, for the first case,

$$\begin{aligned}
\langle \sigma_{m\in A} \sigma_{n\in A} \rangle &= \frac{1}{Z(N,h,T)} \sum_{\sigma_1} \cdots \sum_{\sigma_N} \langle \sigma_1 | P_{AB} | \sigma_2 \rangle \cdots \langle \sigma_{m-1} | P_{BA} | \sigma_m \rangle \sigma_m \langle \sigma_m | P_{AB} | \sigma_{m+1} \rangle \cdots \times \\
&\qquad \cdots \langle \sigma_{n-1} | P_{BA} | \sigma_n \rangle \sigma_n \langle \sigma_n | P_{AB} | \sigma_{n+1} \rangle \cdots \langle \sigma_N | P_{BA} | \sigma_1 \rangle \\
&= \frac{1}{Z(N,h,T)} \sum_{\sigma_1} \langle \sigma_1 | (P_{AA})^{\frac{m-1}{2}} \hat{\sigma}_z (P_{AA})^{\frac{n-m}{2}} \hat{\sigma}_z (P_{AA})^{\frac{N+1-n}{2}} | \sigma_1 \rangle \\
&= \frac{1}{Z(N,h,T)} \mathrm{Tr}\left( (P_{AA})^{\frac{m-1}{2}} \hat{\sigma}_z (P_{AA})^{\frac{n-m}{2}} \hat{\sigma}_z (P_{AA})^{\frac{N+1-n}{2}} \right).
\end{aligned} \tag{25}$$

In the thermodynamic limit $N \to \infty$, for $\lambda_+ > \lambda_- \geq 0$,

$$\langle \sigma_{m\in A}\sigma_{n\in A}\rangle = |\langle \Psi_{A,+}|\hat{\sigma}_z|\Psi_{A,+}\rangle|^2 + \left(\frac{\lambda_-}{\lambda_+}\right)^{\frac{n-m}{2}} |\langle \Psi_{A,-}|\hat{\sigma}_z|\Psi_{A,+}\rangle|^2. \tag{26}$$

(ii) Likewise, for the second case,

$$\langle \sigma_{m\in B}\sigma_{n\in B}\rangle = |\langle \Psi_{B,+}|\hat{\sigma}_z|\Psi_{B,+}\rangle|^2 + \left(\frac{\lambda_-}{\lambda_+}\right)^{\frac{n-m}{2}} |\langle \Psi_{B,-}|\hat{\sigma}_z|\Psi_{B,+}\rangle|^2. \tag{27}$$

(iii) For the third case,

$$\langle \sigma_{m\in A}\sigma_{n\in B}\rangle = \frac{1}{Z(N,h,T)}\mathrm{Tr}\left((P_{AA})^{\frac{m-1}{2}}\hat{\sigma}_z(P_{AA})^{\frac{n-m-1}{2}}P_{AB}\hat{\sigma}_z P_{BA}(P_{AA})^{\frac{N-n}{2}}\right). \tag{28}$$

In the thermodynamic limit $N \to \infty$,

$$\langle \sigma_{m\in A}\sigma_{n\in B}\rangle = \langle \Psi_{A,+}|\hat{\sigma}_z|\Psi_{A,+}\rangle\langle \Psi_{A,+}|\frac{P_{AB}\hat{\sigma}_z P_{BA}}{\lambda_+}|\Psi_{A,+}\rangle + \left(\frac{\lambda_-}{\lambda_+}\right)^{\frac{n-m-1}{2}} \langle \Psi_{A,+}|\hat{\sigma}_z|\Psi_{A,-}\rangle\langle \Psi_{A,-}|\frac{P_{AB}\hat{\sigma}_z P_{BA}}{\lambda_+}|\Psi_{A,+}\rangle. \tag{29}$$

For the nearest neighbor,

$$\langle \sigma_i\sigma_{i+1}\rangle = \frac{1}{\lambda_+}\langle \Psi_{A,+}|\hat{\sigma}_z P_{AB}\hat{\sigma}_z P_{BA}|\Psi_{A,+}\rangle. \tag{30}$$

### C. Sublattice magnetization

$$\begin{aligned}\langle \sigma_{i\in A}\rangle &= \frac{1}{Z(N,h,T)}\sum_{\sigma_1}\cdots\sum_{\sigma_N}\sigma_{i\in A}e^{-\beta H}\\ &= \frac{\mathrm{Tr}\left(\hat{\sigma}_z(P_{AA})^{\frac{N}{2}}\right)}{\mathrm{Tr}\left((P_{AA})^{\frac{N}{2}}\right)}.\end{aligned} \tag{31}$$

In the thermodynamic limit of $N \to \infty$, for $\lambda_+ > \lambda_- \geq 0$,

$$\langle \sigma_{i\in A}\rangle = \langle \Psi_{A,+}|\hat{\sigma}_z|\Psi_{A,+}\rangle \tag{32}$$

$$\langle \sigma_{i\in B}\rangle = \langle \Psi_{B,+}|\hat{\sigma}_z|\Psi_{B,+}\rangle \tag{33}$$

### D. The zero-temperature limit

We focus on the $Jg_Ag_B < 0$ case of current interest.

#### 1. $-g_B > g_A > 0$

Firstly, for nonuniform $g$-factors, either $\frac{|g_A+g_B|h}{T} \to \infty$ or $\frac{|g_A-g_B|h}{T} \to \infty$. Without loss of generality, we study $J > 0$ and $-g_B > g_A > 0$, i.e., $\frac{(g_A+g_B)h}{T} \to -\infty$ and $\frac{(g_A-g_B)h}{T} \to \infty$. Then,

$$\begin{aligned}\lambda_+ &= 2e^{\beta h|g_B|}\cosh[\beta(h_c-h)g_A],\\ f(h,T\to 0) &= -\frac{k_\mathrm{B}T}{2}\ln 2 - h\frac{|g_B|}{2} - \frac{k_\mathrm{B}T}{2}\ln[\cosh(\frac{h_c-h}{k_\mathrm{B}T}g_A)],\\ m(h,T\to 0) &= \frac{|g_B|}{2} - \frac{g_A}{2}\tanh(\frac{h_c-h}{k_\mathrm{B}T}g_A)\\ S(h,T\to 0) &= \frac{k_\mathrm{B}}{2}\ln 2 + \frac{k_\mathrm{B}}{2}\ln[\cosh(\frac{h_c-h}{k_\mathrm{B}T}g_A)] - \frac{h_c-h}{2T}g_A\tanh(\frac{h_c-h}{k_\mathrm{B}T}g_A)\end{aligned} \tag{34}$$

with the critical field $h_c = 2J/g_A$. More specifically,

$$m(h, T \to 0) = \begin{cases} \frac{1}{2}(|g_B| - g_A) & 0 < h < h_c \\ \frac{1}{2}|g_B| \quad \text{for} & h = h_c \\ \frac{1}{2}(|g_B| + g_A) & h > h_c \end{cases} \tag{35}$$

$$S(h, T \to 0) = \begin{cases} 0 & 0 < h < h_c \\ \frac{1}{2}k_{\rm B}\ln 2 \quad \text{for} & h = h_c \\ 0 & h > h_c \end{cases} \tag{36}$$

The eigenvectors are

$$\begin{aligned} |\Psi_{A,+}\rangle &= \begin{pmatrix} e^{-\beta g_A(h_c-h)/2} \\ e^{\beta g_A(h_c-h)/2} \end{pmatrix}, \qquad |\Psi_{B,+}\rangle = \begin{pmatrix} 0 \\ 1 \end{pmatrix} \\ |\Psi_{A,-}\rangle &= \begin{pmatrix} e^{\beta g_A(h_c-h)/2} \\ -e^{-\beta g_A(h_c-h)/2} \end{pmatrix}, \qquad |\Psi_{B,-}\rangle = \begin{pmatrix} 1 \\ 0 \end{pmatrix} \end{aligned} \tag{37}$$

subject to normalization. We arrive at

$$\begin{aligned} \langle\sigma_{i\in A}\rangle &= -\tanh[\beta g_A(h_c - h)], \\ \langle\sigma_{i\in B}\rangle &= -1, \\ \langle\sigma_i\sigma_{i+1}\rangle &= \tanh[\beta g_A(h_c - h)]. \end{aligned} \tag{38}$$

More specifically, for $0 < h < h_c$,

$$\begin{aligned} |\Psi_{A,+}\rangle &= \begin{pmatrix} 0 \\ 1 \end{pmatrix}, \qquad |\Psi_{B,+}\rangle = \begin{pmatrix} 0 \\ 1 \end{pmatrix} \\ |\Psi_{A,-}\rangle &= \begin{pmatrix} 1 \\ 0 \end{pmatrix}, \qquad |\Psi_{B,-}\rangle = \begin{pmatrix} 1 \\ 0 \end{pmatrix} \end{aligned} \tag{39}$$

$$\begin{aligned} \langle\sigma_{i\in A}\rangle &= -1, \\ \langle\sigma_{i\in B}\rangle &= -1, \\ \langle\sigma_i\sigma_{i+1}\rangle &= 1. \end{aligned} \tag{40}$$

That is, the ground state of the system is $|-\,-\,-\,-\,-\,-\,-\,-\,-\cdots\rangle$, which gains energy from both the $J$ and $h$ terms.

For $h = h_c$,

$$\begin{aligned} |\Psi_{A,+}\rangle &= \frac{1}{\sqrt{2}}\begin{pmatrix} 1 \\ 1 \end{pmatrix}, \qquad |\Psi_{B,+}\rangle = \begin{pmatrix} 0 \\ 1 \end{pmatrix} \\ |\Psi_{A,-}\rangle &= \frac{1}{\sqrt{2}}\begin{pmatrix} -1 \\ 1 \end{pmatrix}, \qquad |\Psi_{B,-}\rangle = \begin{pmatrix} 1 \\ 0 \end{pmatrix} \end{aligned} \tag{41}$$

$$\begin{aligned} \langle\sigma_{i\in A}\rangle &= 0, \\ \langle\sigma_{i\in B}\rangle &= -1, \\ \langle\sigma_i\sigma_{i+1}\rangle &= 0, \end{aligned} \tag{42}$$

which gains energy from $h$ term but nothing from the $J$ term.

For $h > h_c$,

$$\begin{aligned} |\Psi_{A,+}\rangle &= \begin{pmatrix} 1 \\ 0 \end{pmatrix}, \qquad |\Psi_{B,+}\rangle = \begin{pmatrix} 0 \\ 1 \end{pmatrix} \\ |\Psi_{A,-}\rangle &= \begin{pmatrix} 0 \\ 1 \end{pmatrix}, \qquad |\Psi_{B,-}\rangle = \begin{pmatrix} 1 \\ 0 \end{pmatrix} \end{aligned} \tag{43}$$

$$\begin{aligned} \langle\sigma_{i\in A}\rangle &= 1, \\ \langle\sigma_{i\in B}\rangle &= -1, \\ \langle\sigma_i\sigma_{i+1}\rangle &= -1. \end{aligned} \tag{44}$$

That is, the ground state of the system is $|+-+-+-+-\cdots\rangle$, which gains energy from the $h$ term to overcome the energy cost from the $J$ term.

### 2. $-g_B = g_A$

In comparison, for $J > 0$ and $-g_B = g_A = g > 0$, i.e., $\frac{(g_A+g_B)h}{T} = 0$ and $\frac{(g_A-g_B)h}{T} \to \infty$. Then,

$$\begin{aligned}
\lambda_+ &= = \frac{1}{4}e^{-2\beta(J-hg)}(1+\Delta)^2 \\
f(h,T) &= J - hg + k_\mathrm{B}T\ln 2 - k_\mathrm{B}T\ln(1+\Delta), \\
m(h,T) &= g\left[1 - \frac{4e^{2\beta g(h_c-h)}}{(1+\Delta)\Delta}\right] \\
S(h,T) &= -\ln 2 + \ln(1+\Delta) + \frac{4\beta g(h_c-h)e^{2\beta g(h_c-h)}}{(1+\Delta)\Delta},
\end{aligned} \tag{45}$$

where

$$\Delta = \sqrt{1+4e^{2\beta g(h_c-h)}} = \begin{cases} 2e^{\beta g(h_c-h)} & 0 < h < h_c \\ \sqrt{5} \quad \text{for} & h = h_c \\ 1 & h > h_c \end{cases} \tag{46}$$

with the critical field $h_c = 2J/g$. More specifically,

$$m(h, T\to 0) = \begin{cases} 0 & 0 < h < h_c \\ g\,\frac{1}{\sqrt{5}} \approx 0.447214\, g \quad \text{for} & h = h_c \\ g & h > h_c \end{cases} \tag{47}$$

$$S(h, T\to 0) = \begin{cases} 0 & 0 < h < h_c \\ k_\mathrm{B}\ln\left(\frac{1+\sqrt{5}}{2}\right) \approx 0.694242\, k_\mathrm{B}\ln 2 \quad \text{for} & h = h_c \\ 0 & h > h_c \end{cases} \tag{48}$$

For $0 \le h < h_c$,

$$\begin{aligned}
\langle\sigma_i\rangle &= 0, \\
\langle\sigma_i\sigma_j\rangle &= 1
\end{aligned} \tag{49}$$

That is, the ground state of the system is $\frac{1}{\sqrt{2}}(|+++++++++\cdots\rangle + |---------\cdots\rangle)$, which gains energy from the $J$ term but nothing from the $h$ term.

For $h = h_c$,

$$\begin{aligned}
\langle\sigma_{i\in A}\rangle &= \frac{1}{\sqrt{5}}, \\
\langle\sigma_{i\in B}\rangle &= -\frac{1}{\sqrt{5}}, \\
\langle\sigma_i\sigma_{i+1}\rangle &= 1 - \frac{2}{\sqrt{5}} \approx 0.1055728,
\end{aligned} \tag{50}$$

which gains energy from both the $J$ and $h$ terms.

For $h > h_c$,

$$\begin{aligned}
\langle\sigma_{i\in A}\rangle &= 1, \\
\langle\sigma_{i\in B}\rangle &= -1, \\
\langle\sigma_{i\in A}\sigma_{j\in B}\rangle &= -1
\end{aligned} \tag{51}$$

That is, the ground state of the system is $|+-+-+-+-\cdots\rangle$, which gains energy from the $h$ term to overcome the energy cost from the $J$ term.

---

* wyin@bnl.gov

[1] J. Kanamori, Progress of Theoretical Physics **17**, 177 (1957), http://ptp.oxfordjournals.org/content/17/2/177.full.pdf+html.
[2] W.-G. Yin, X. Liu, A. M. Tsvelik, M. P. M. Dean, M. H. Upton, J. Kim, D. Casa, A. Said, T. Gog, T. F. Qi, G. Cao, and J. P. Hill, Phys. Rev. Lett. **111**, 057202 (2013).
[3] D. C. Mattis and R. H. Swendsen, *Statistical Mechanics Made Simple* (World Scientific Publishing Company, 2008).
